# Supplementary material for: Measurement of the differential cross section for neutral pion production in charged-current muon neutrino interactions on argon with the MicroBooNE detector
Source: arXiv:2404.09949 ancillary file (2024-05-06)
Supplement: Supplementary file 1 [file Supplemental_Material.pdf]

## 2 Supplemental Material: Measurement of the differential cross section for neutral pion 3 production in charged-current muon neutrino interactions on argon with the 4 MicroBooNE detector

5 The supplemental material contains more details about the results presented in the main text for the  $\nu_\mu$  CC1 $\pi^0$  dif-  
6 ferential cross section measurement. The following sections include the ingredients to reproduce the single differential  
7 cross section for each of the five kinematic variables.

### 8 I. EFFICIENCIES : MUON, CHARGED PION KINETIC ENERGY

9 Figure 1 shows the reconstruction efficiencies for the  $\nu_\mu$  CC1 $\pi^0$  selection as a function of the muon and charged pion  
10 kinetic energies. Phase space cuts used as signal definition in this analysis are placed in regions without significant  
11 slope. The lower efficiency at high charged pion kinetic energy implies that our selection is able to veto charged pions  
12 more effectively in this region.

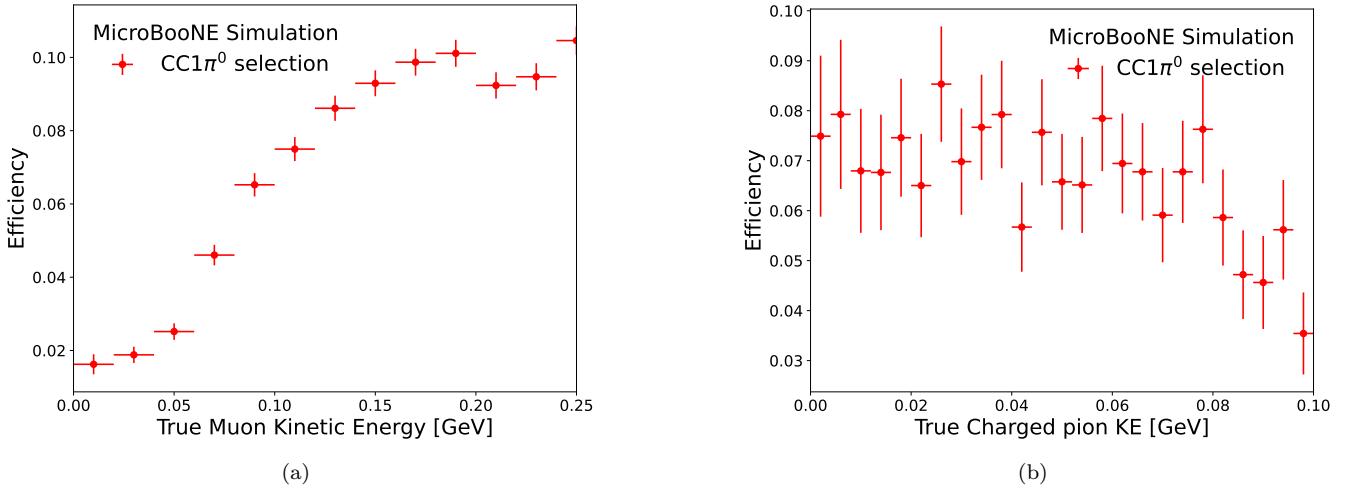

13 FIG. 1. Efficiency as a function of (a) the muon kinetic energy, and (b) the charged pion kinetic energy for the  $\nu_\mu$  CC1 $\pi^0$   
14 selection are shown.

### 15 II. INTERACTION MODES OF SELECTED EVENTS

16 The distribution of the predicted signal events passing the  $\nu_\mu$  CC1 $\pi^0$  selection criteria classified by true interaction  
17 mode for the tuned version of GENIE v3 is shown in Fig. 2.

### 19 III. NUMBER OF TARGETS USED IN CROSS SECTION EXTRACTION

20 Calculating the total number of nucleon targets is a matter of counting, and is done by multiplying the number of  
21 nucleons in one argon nucleus by the number of argon nuclei we expect to be present in the fiducial volume of the  
22 detector used to conduct the measurement. The fiducial volume coordinates used in this analysis are given below,

$$\begin{aligned} 8.45\text{cm} &\leq x \leq 244.8\text{cm} \\ -100.53\text{cm} &\leq y \leq 102.47\text{cm} \\ 10.1\text{cm} &\leq z \leq 986.9\text{cm} \end{aligned}$$

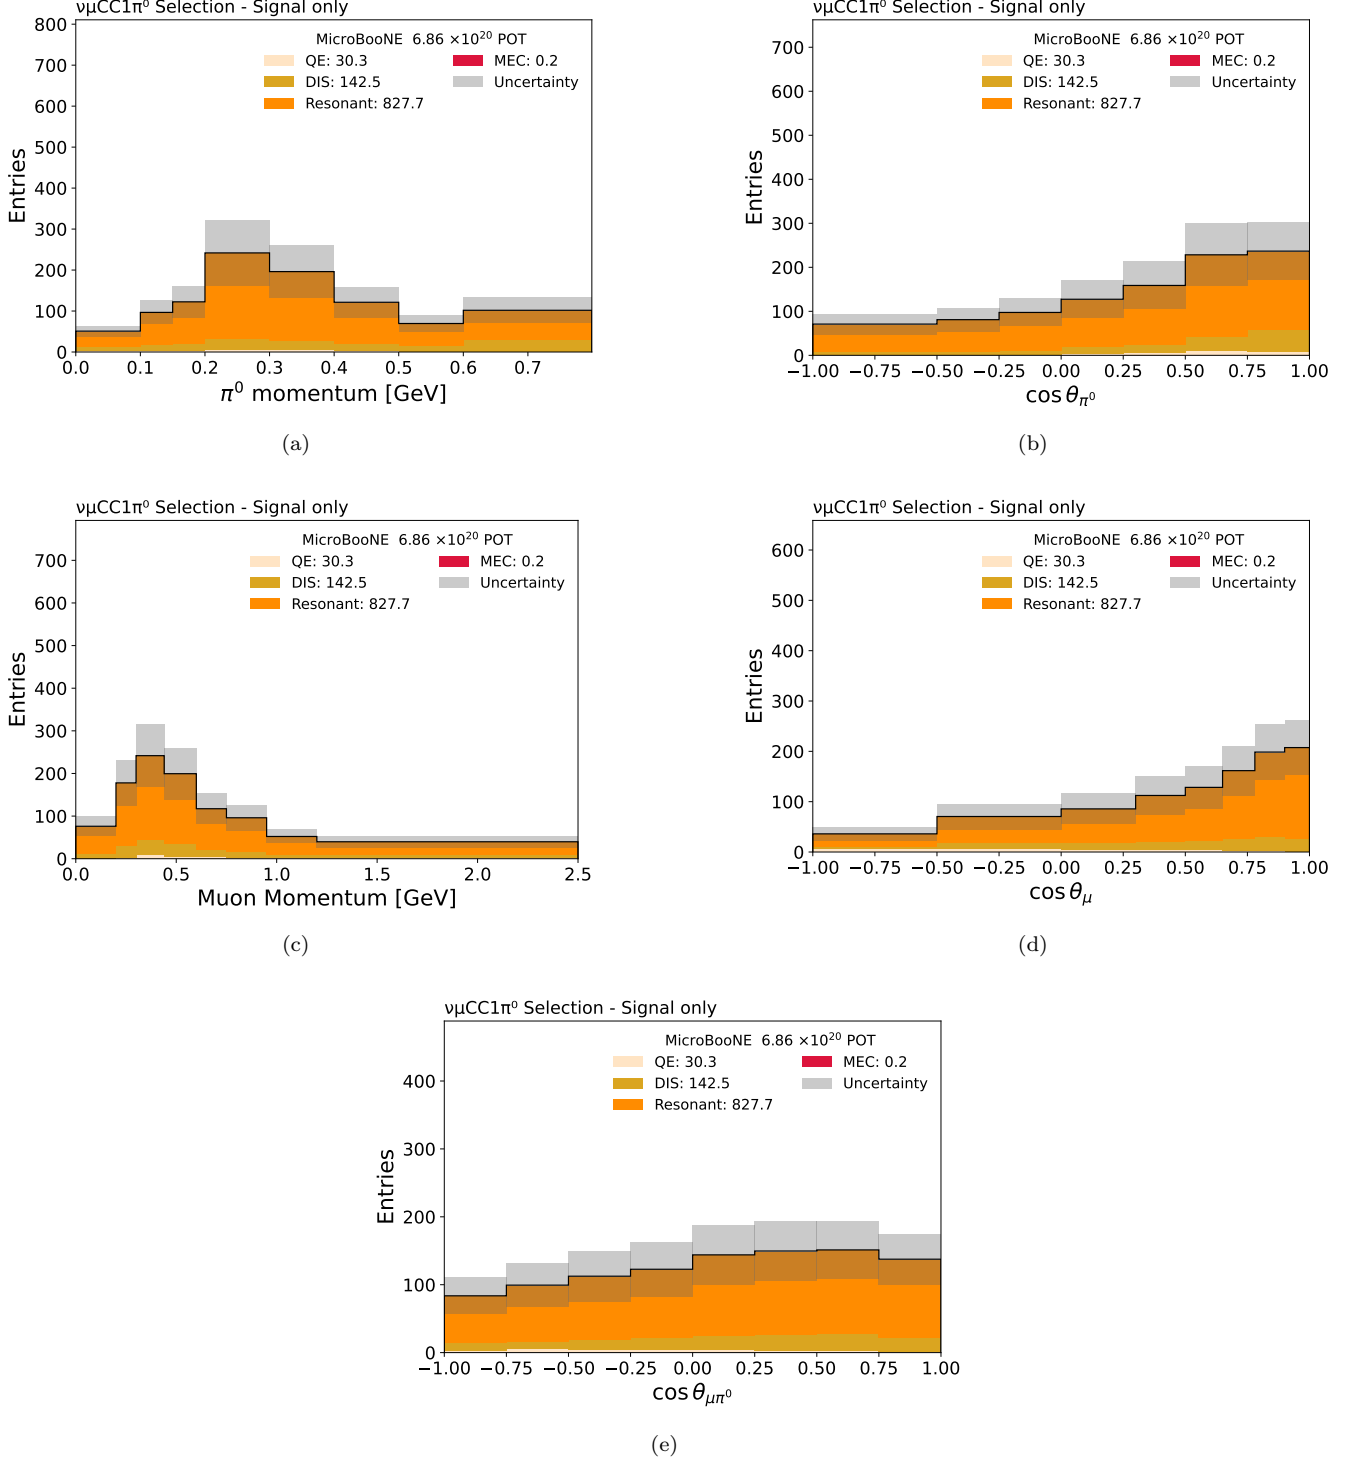

FIG. 2. The distribution of the signal prediction using the MicroBooNE tune of GENIE v3 after  $\nu_{\mu}$  CC1 $\pi^0$  selection, categorized by interaction mode is shown for (a) the  $\pi^0$  momentum, (b) the scattering angle between the neutrino beam and outgoing  $\pi^0$  direction, (c) the muon momentum, (d) the scattering angle between the neutrino beam and outgoing muon direction, and (e) the opening angle between the muon and pion. The interaction categories in the legend shows quasielastic (QE), meson exchange current (MEC), resonant, and deep inelastic scattering (DIS) contributions.

<sup>23</sup> The coordinates above have 10 cm, 15 cm and 10(50) cm offsets in the x, y and z direction respectively from the  
<sup>24</sup> boundaries of the TPC active volume. Events with a neutrino vertex within the fiducial volume defined above are

considered as signal.

$$N_{targets} = \frac{\rho_{Ar} \times V \times N_A \times N_{nucleons}}{m_{mol}} = 9.75 \times 10^{29} \quad (1)$$

where  $\rho_{Ar}$  is the density of liquid argon,  $V$  is the volume of liquid argon,  $N_A$  is Avogadro's number,  $N_{nucleons}$  is the number of nucleons in an argon nucleus, and  $m_{mol}$  is the molar mass of argon. The flux prediction can be found in the supplemental material of [1].

#### IV. TOTAL FLUX INTEGRATED CROSS SECTION

We report the flux-integrated total  $\nu_\mu$  CC1 $\pi^0$  cross section for this analysis to be  $\sigma = (5.42 \pm 1.09) \times 10^{-40} \text{cm}^2/\text{nucleon}$ . This is consistent with the previous MicroBooNE measurement reported in [2].

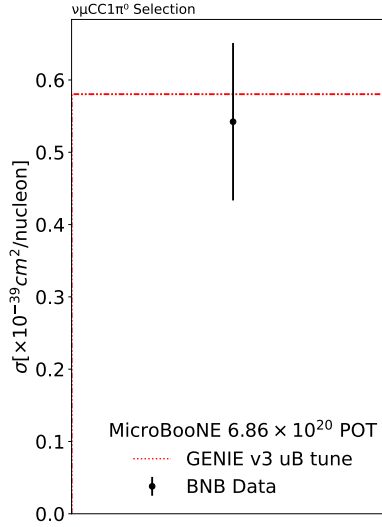

FIG. 3. The data extracted total flux integrated  $\nu_\mu$  CC1 $\pi^0$  cross section is compared to the tuned version of the GENIE prediction. The error bar on the data includes both statistical and systematic uncertainties.

#### V. $\pi^0$ MOMENTUM

We provide additional information for the cross section measurement as a function of  $\pi^0$  momentum: the number of total selected events, background-subtracted observed events and the total covariance matrix, response matrix, unfolded central value cross section values and covariance, and the additional smearing matrix  $A_c$  returned by the Wiener-SVD method. Comparisons with generators are performed after applying  $A_c$  to all predictions. The last bin in the  $\pi^0$  momentum distribution includes all overflow events.

| $\pi^0$ Momentum [GeV/c]                                                              | [0.0, 0.1] | [0.1, 0.15] | [0.15, 0.2] | [0.2, 0.3] | [0.3, 0.4] | [0.4, 0.5] | [0.5, 0.6] | [0.6, 0.799] |
|---------------------------------------------------------------------------------------|------------|-------------|-------------|------------|------------|------------|------------|--------------|
| Background-subtracted data events                                                     | 69.606     | 116.158     | 157.998     | 226.806    | 152.219    | 91.121     | 40.639     | 91.219       |
| Unfolded cross section<br>[ $\times 10^{-39} \text{cm}^2/\text{GeV}/\text{nucleon}$ ] | 0.66       | 1.92        | 2.44        | 1.15       | 0.73       | 0.34       | 0.18       | 0.09         |

TABLE I. Numbers of background-subtracted data events and unfolded cross section as a function of  $\pi^0$  momentum.

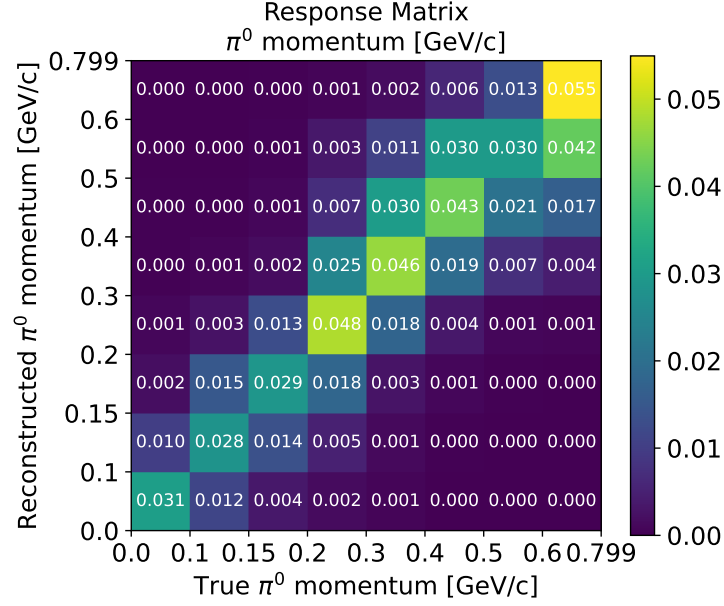

FIG. 4. The response matrix used as an input to the Wiener-SVD unfolding algorithm as a function of reconstructed and true  $\pi^0$  momentum is constructed using the signal prediction obtained with GENIE v3.0.6 G18\_10a\_02\_11a [3] after applying the selection.

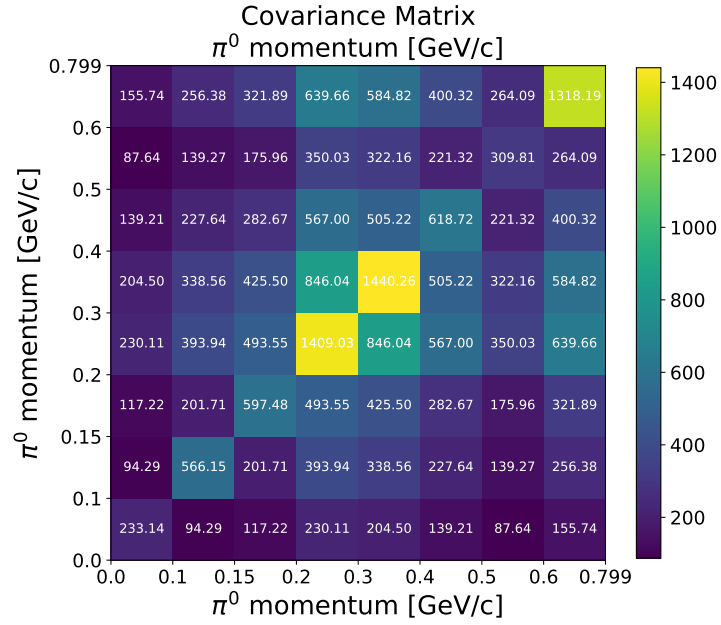

FIG. 5. Covariance matrix for the total event prediction as a function of  $\pi^0$  momentum.

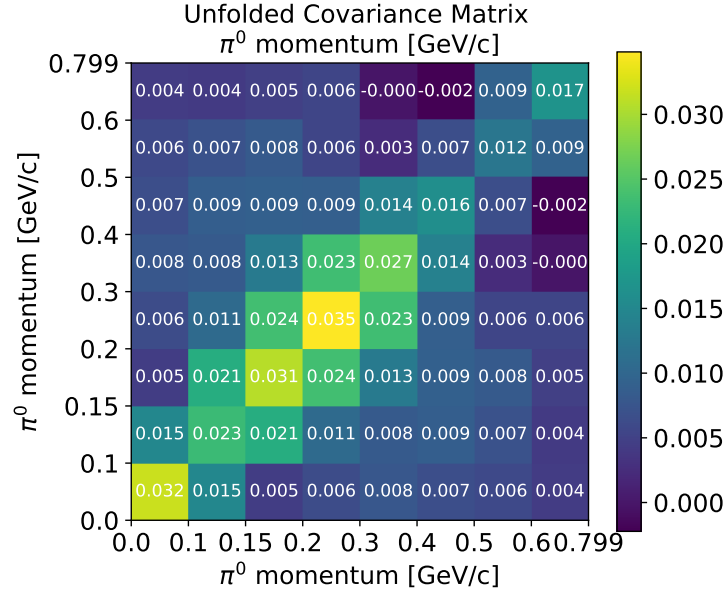

FIG. 6. Unfolded covariance of the cross section result as a function of  $\pi^0$  momentum, in units of  $(10^{-40} \text{ cm}^2/\text{GeV/nucleon})^2$ .

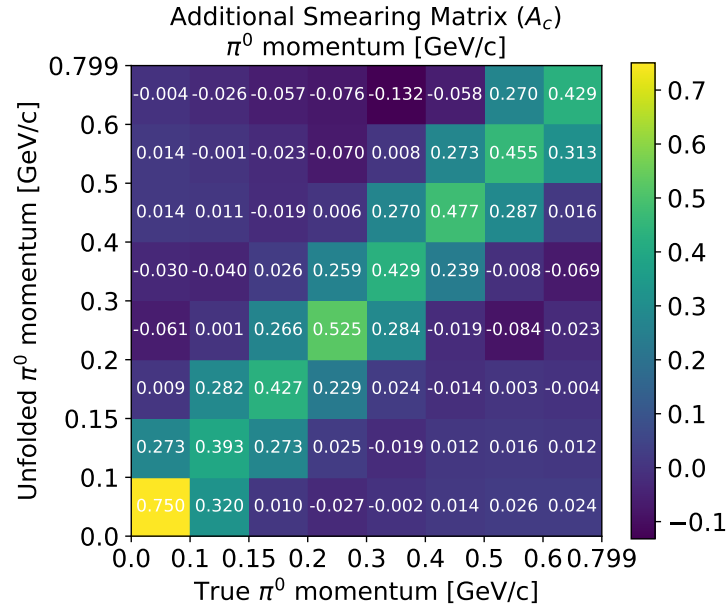

FIG. 7. The additional smearing matrix  $A_c$  returned by the Wiener-SVD method for unfolded  $\pi^0$  momentum, which is used to smear the generator predictions and to compare with the data extracted cross section into the unfolded space.

## VI. $\pi^0$ ANGLE

We provide additional information for the cross section measurement as a function of  $\pi^0$  angle: the number of total selected events, background-subtracted observed events and the total covariance matrix, response matrix, unfolded central value cross section values and covariance, and the additional smearing matrix  $A_c$  returned by the Wiener-SVD method. Comparisons with generators are performed after applying  $A_c$  to all predictions.

| $\pi^0$ angle                                                           | [-1.0, -0.5] | [-0.5, -0.25] | [-0.25, 0.0] | [0.0, 0.25] | [0.25, 0.5] | [0.5, 0.75] | [0.75, 1.0] |
|-------------------------------------------------------------------------|--------------|---------------|--------------|-------------|-------------|-------------|-------------|
| Background-subtracted data events                                       | 48.39        | 72.274        | 101.453      | 110.648     | 158.815     | 224.717     | 229.469     |
| Unfolded cross section<br>[ $\times 10^{-39}$ cm <sup>2</sup> /nucleon] | 0.10         | 0.17          | 0.20         | 0.19        | 0.23        | 0.40        | 0.49        |

TABLE II. Numbers of background-subtracted data events and unfolded cross section as a function of  $\pi^0$  angle.

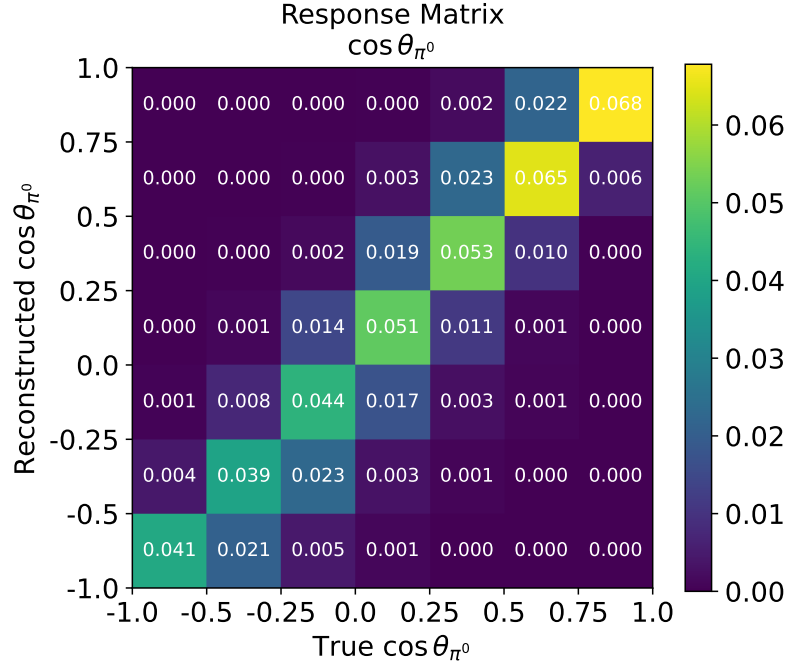

FIG. 8. The response matrix used as an input to the Wiener-SVD unfolding algorithm as a function of reconstructed and true  $\pi^0$  angle is constructed using the signal prediction obtained with GENIE v3.0.6 G18\_10a.02.11a [3] after applying the selection.

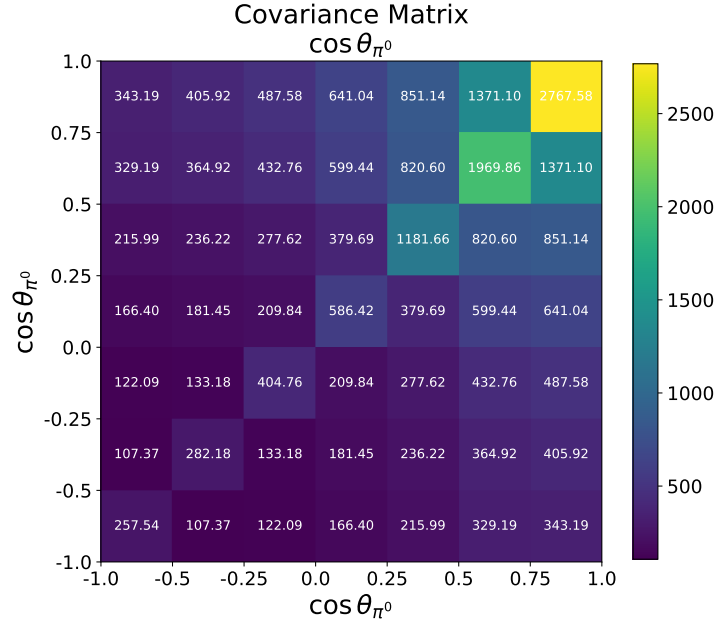

FIG. 9. Covariance matrix for the total event prediction as a function of  $\pi^0$  angle.

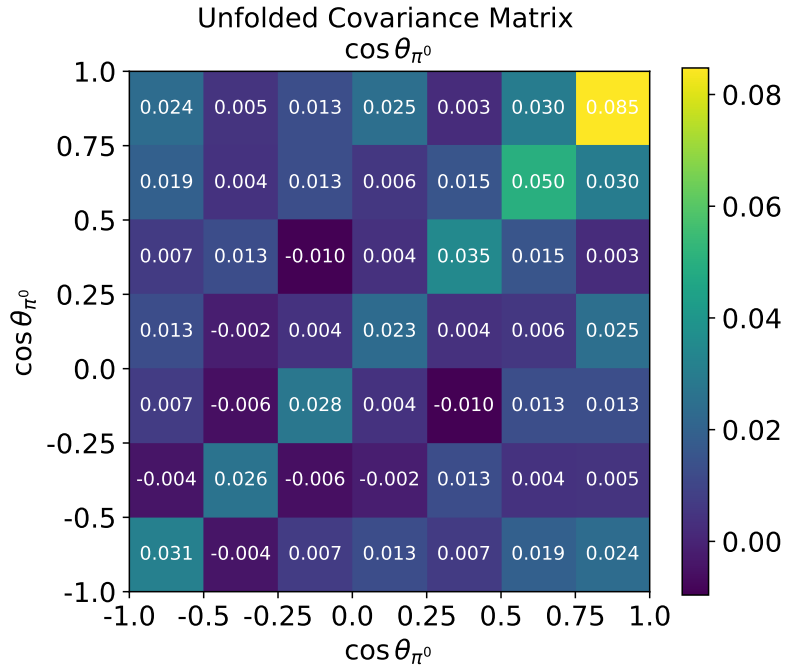

FIG. 10. Unfolded covariance of the cross section result as a function of  $\pi^0$  angle, in units of  $(10^{-40} \text{ cm}^2/\text{nucleon})^2$ .

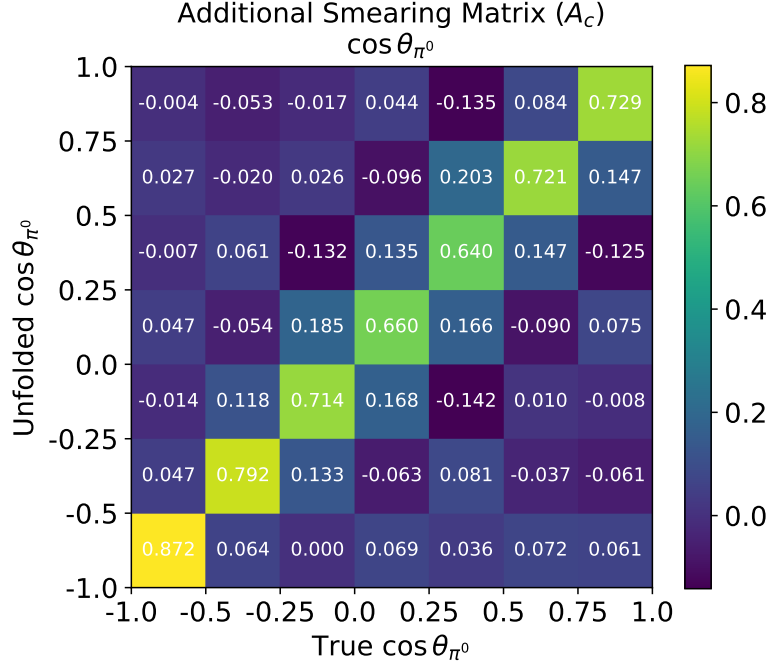

FIG. 11. The additional smearing matrix  $A_c$  returned by the Wiener-SVD method for unfolded  $\pi^0$  angle, which is used to smear the generator predictions and to compare with the data extracted cross section into the unfolded space.

## VII. MUON MOMENTUM

We provide additional information for the cross section measurement as a function of muon momentum: the number of total selected events, background-subtracted observed events and the total covariance matrix, response matrix, unfolded central value cross section values and covariance, and the additional smearing matrix  $A_c$  returned by the Wiener-SVD method. Comparisons with generators are performed after applying  $A_c$  on all predictions. The last bin in the muon momentum distribution includes all overflow events.

| muon Momentum [GeV/c]                                                       | [0.0, 0.2] | [0.2, 0.3] | [0.3, 0.44] | [0.44, 0.6] | [0.6, 0.75] | [0.75, 0.95] | [0.95, 1.2] | [1.2, 2.5] |
|-----------------------------------------------------------------------------|------------|------------|-------------|-------------|-------------|--------------|-------------|------------|
| Background-subtracted data events                                           | 77.254     | 209.492    | 286.565     | 181.499     | 108.765     | 55.109       | 17.274      | 9.858      |
| Unfolded cross section<br>[ $\times 10^{-39}$ cm <sup>2</sup> /GeV/nucleon] | 0.45       | 1.08       | 0.79        | 0.57        | 0.43        | 0.16         | 0.05        | 0.005      |

TABLE III. Numbers of background-subtracted data events and unfolded cross section as a function of muon momentum.

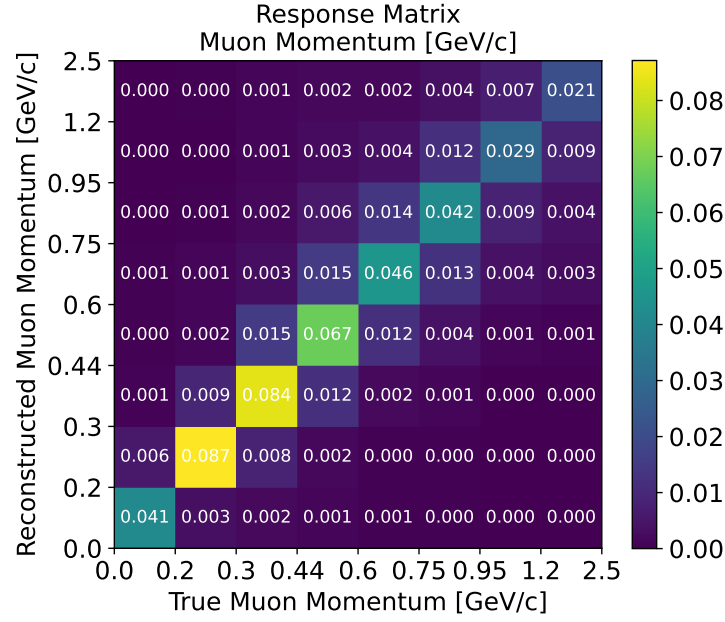

FIG. 12. The response matrix used as an input to the Wiener-SVD unfolding algorithm as a function of reconstructed and true muon momentum is constructed using the signal prediction obtained with GENIE v3.0.6 G18\_10a\_02\_11a [3] after applying the selection.

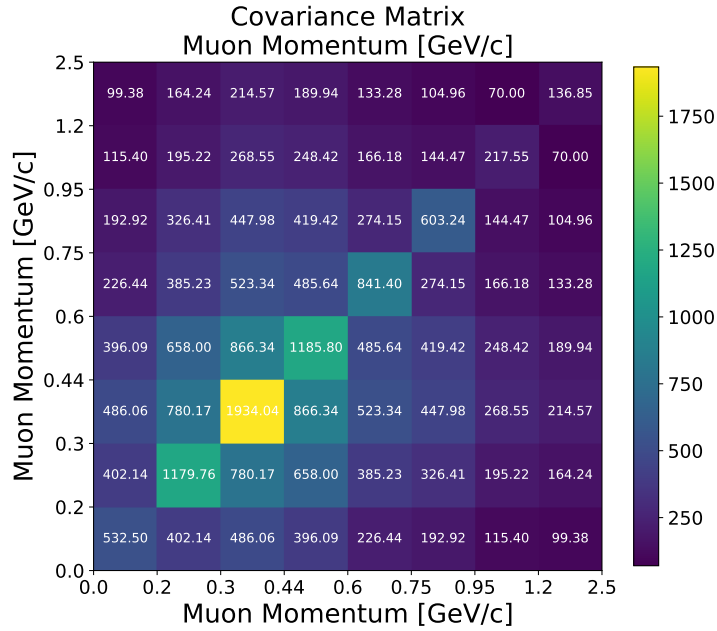

FIG. 13. Covariance matrix for the total event prediction as a function of muon momentum.

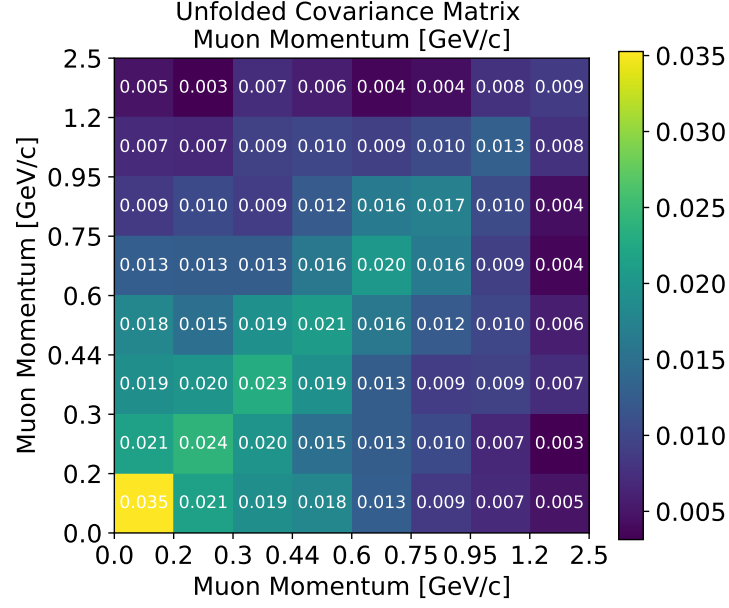

FIG. 14. Unfolded covariance of the cross section result as a function of muon momentum, in units of  $(10^{-40} \text{ cm}^2/\text{GeV}/\text{nucleon})^2$ .

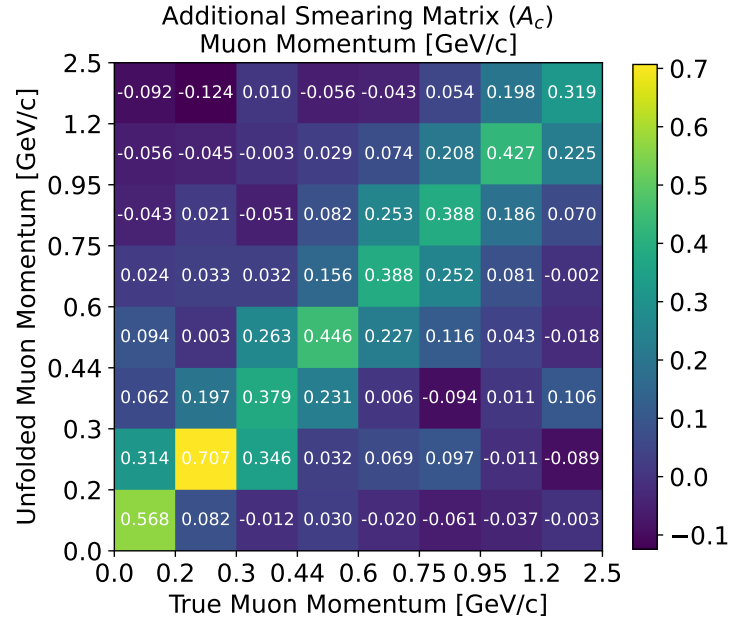

FIG. 15. The additional smearing matrix  $A_c$  returned by the Wiener-SVD method for unfolded muon momentum, which is used to smear the generator predictions and to compare with the data extracted cross section into the unfolded space.

# VIII. MUON ANGLE

We provide additional information for the cross section measurement as a function of muon angle: the number of total selected events, background-subtracted observed events and the total covariance matrix, response matrix, unfolded central value cross section values and covariance, and the additional smearing matrix  $A_c$  returned by the Wiener-SVD method. Comparisons with generators are performed after applying  $A_c$  on all predictions.

| $\cos(\theta_\mu)$                                                      | [-1.0, -0.5] | [-0.5, 0.0] | [0.0, 0.3] | [0.3, 0.5] | [0.5, 0.65] | [0.65, 0.78] | [0.78, 0.9] | [0.9, 1.0] |
|-------------------------------------------------------------------------|--------------|-------------|------------|------------|-------------|--------------|-------------|------------|
| Background-subtracted data events                                       | 46.665       | 81.967      | 92.635     | 128.674    | 140.998     | 149.282      | 170.028     | 135.515    |
| Unfolded cross section<br>[ $\times 10^{-39}$ cm <sup>2</sup> /nucleon] | 0.06         | 0.11        | 0.19       | 0.29       | 0.43        | 0.48         | 0.66        | 0.65       |

TABLE IV. Numbers of background-subtracted data events and unfolded cross section as a function of muon angle.

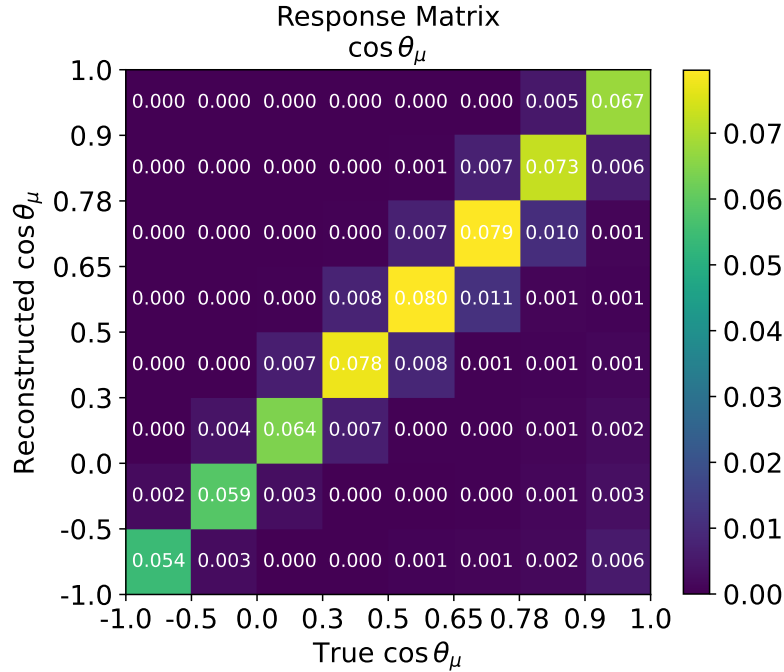

FIG. 16. The response matrix used as an input to the Wiener-SVD unfolding algorithm as a function of reconstructed and true muon angle is constructed using the signal prediction obtained with GENIE v3.0.6 G18\_10a\_02\_11a [3] after applying the selection.

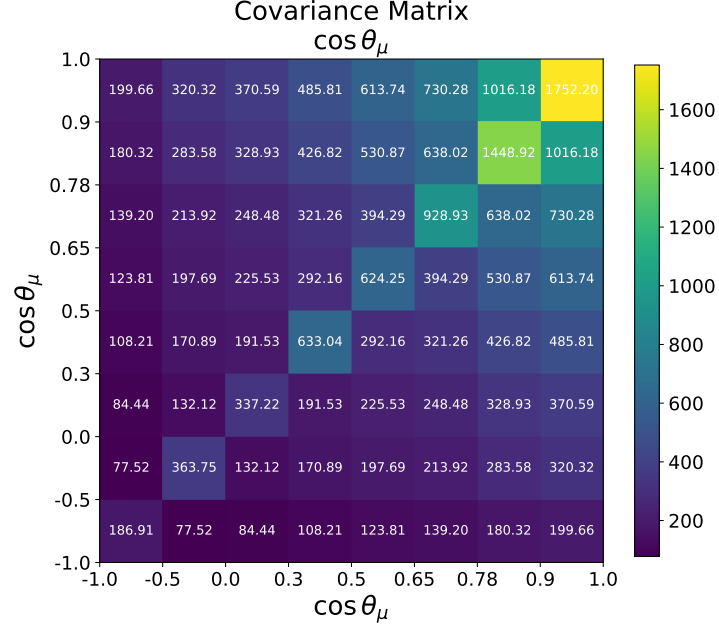

FIG. 17. Covariance matrix for the total event prediction as a function of muon angle.

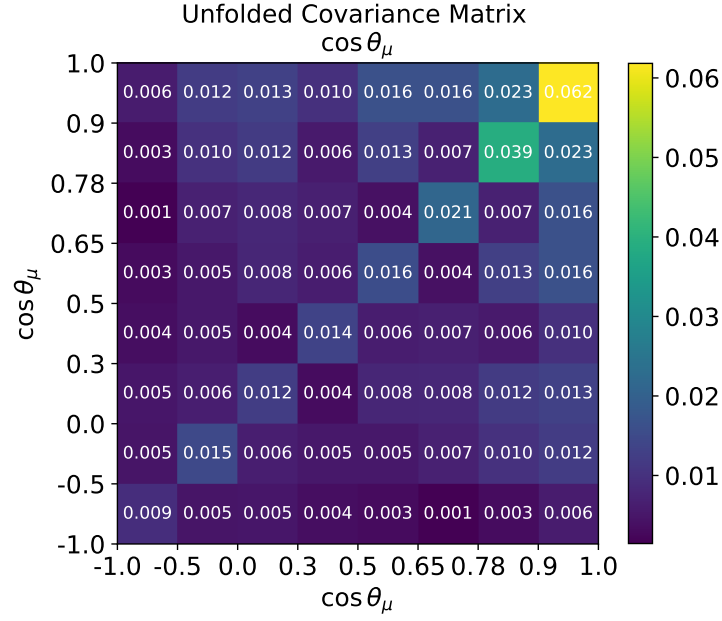

FIG. 18. Unfolded covariance of the cross section result as a function of muon angle, in units of  $(10^{-40} \text{ cm}^2/\text{nucleon})^2$ .

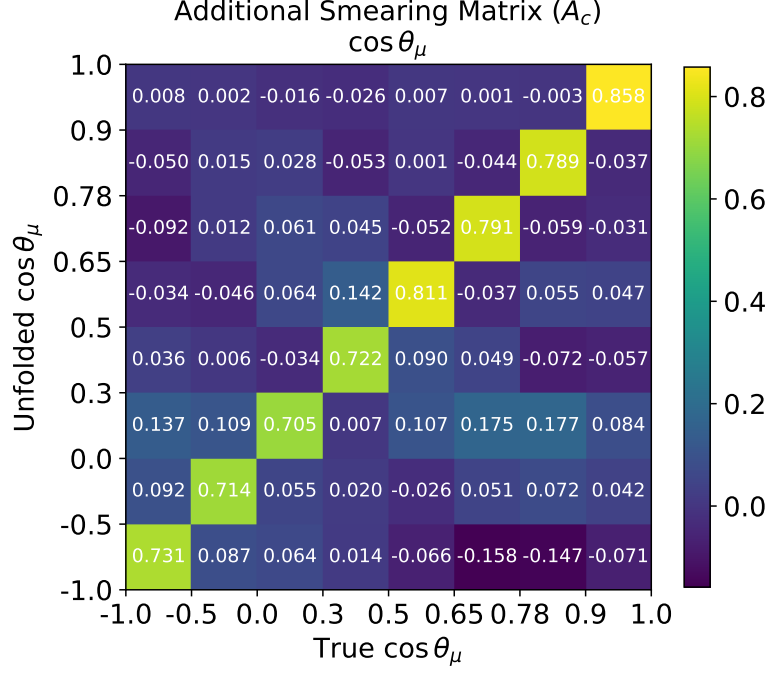

FIG. 19. The additional smearing matrix  $A_c$  returned by the Wiener-SVD method for unfolded muon angle, which is used to smear the generator predictions and to compare with the data extracted cross section into the unfolded space.

## IX. MUON PION OPENING ANGLE

We provide additional information for the cross section measurement as a function of the muon pion opening angle: the number of total selected events, background-subtracted observed events and the total covariance matrix, response matrix, unfolded central value cross section values and covariance, and the additional smearing matrix  $A_c$  returned by the Wiener-SVD method. Comparisons with generators are performed after applying  $A_c$  on all predictions.

| $\cos(\theta_{\mu\pi^0})$                                               | [-1.0, -0.75] | [-0.75, -0.5] | [-0.5, -0.25] | [-0.25, 0.0] | [0.0, 0.25] | [0.25, 0.5] | [0.5, 0.75] | [0.75, 1.0] |
|-------------------------------------------------------------------------|---------------|---------------|---------------|--------------|-------------|-------------|-------------|-------------|
| Background-subtracted data events                                       | 93.519        | 88.728        | 99.759        | 132.945      | 139.408     | 129.693     | 128.365     | 133.349     |
| Unfolded cross section<br>[ $\times 10^{-39}$ cm <sup>2</sup> /nucleon] | 0.25          | 0.19          | 0.22          | 0.28         | 0.28        | 0.24        | 0.26        | 0.23        |

TABLE V. Numbers of background-subtracted data events and unfolded cross section as a function of muon pion opening angle.

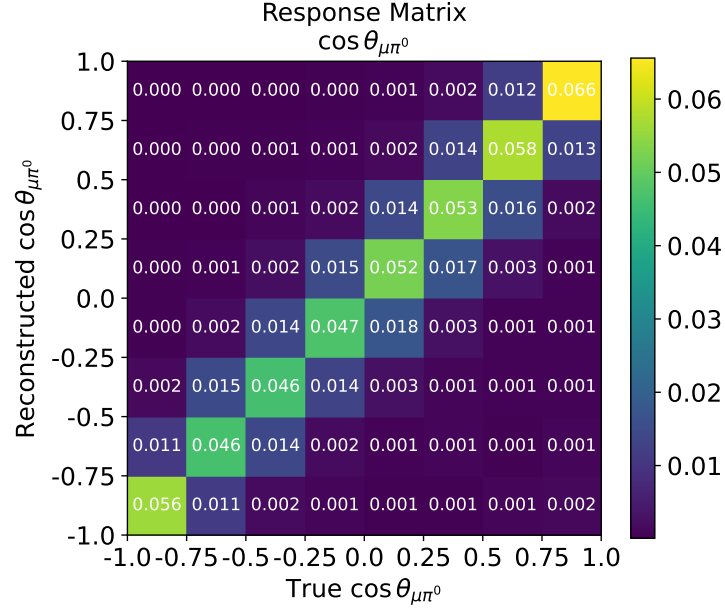

FIG. 20. The response matrix used as an input to the Wiener-SVD unfolding algorithm as a function of reconstructed and true muon pion opening angle is constructed using the signal prediction obtained with GENIE v3.0.6 G18\_10a\_02\_11a [3] after applying the selection.

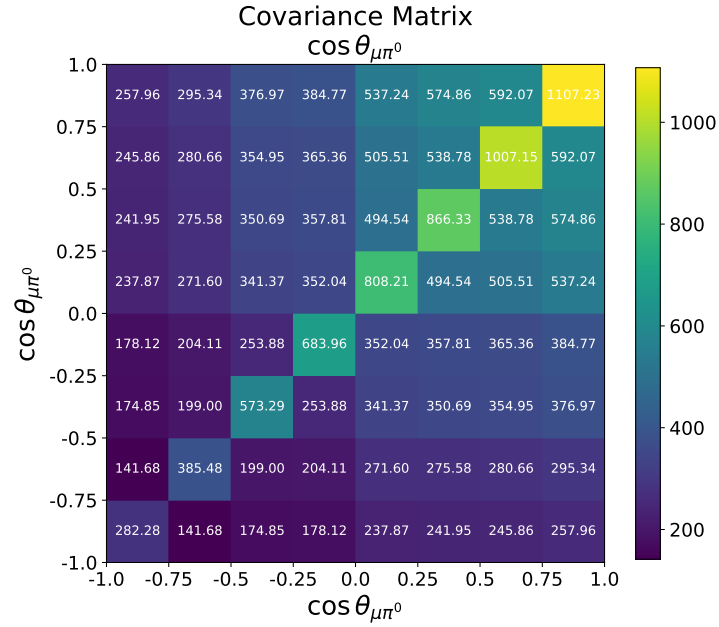

FIG. 21. Covariance matrix for the total event prediction as a function of the muon pion opening angle.

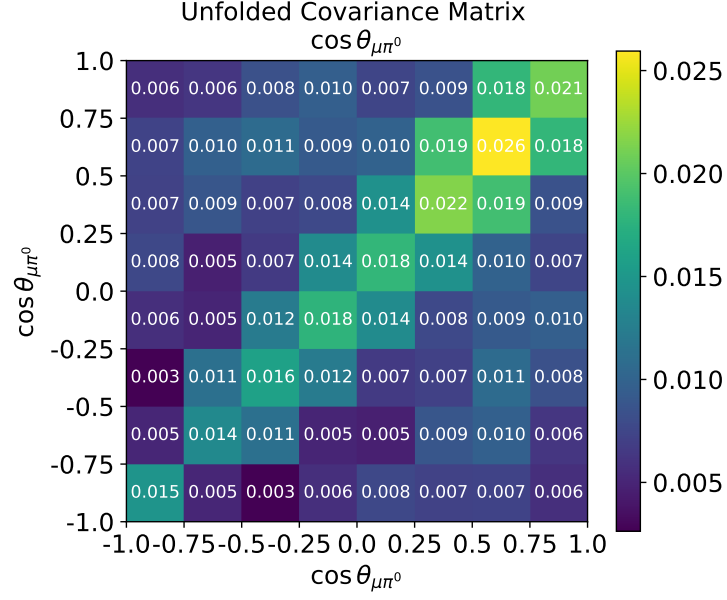

FIG. 22. Unfolded covariance of the cross section result as a function of the muon pion opening angle, in units of  $(10^{-40} \text{ cm}^2/\text{nucleon})^2$ .

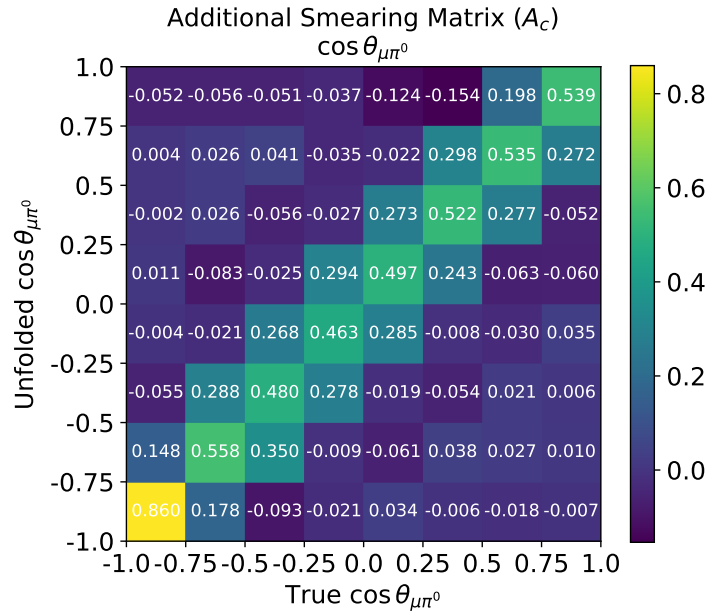

FIG. 23. The additional smearing matrix  $A_c$  returned by the Wiener-SVD method for the unfolded muon pion opening angle, which is used to smear the generator predictions and to compare with the data extracted cross section into the unfolded space.

## X. FSI EFFECTS

In this section we focus on understanding the FSI effects when we compare the data extracted cross section with the generator predictions. The plots include generator predictions with FSI effects turned off. The  $\chi^2/ndf$  for each of the cases are included in the legend of the plots.

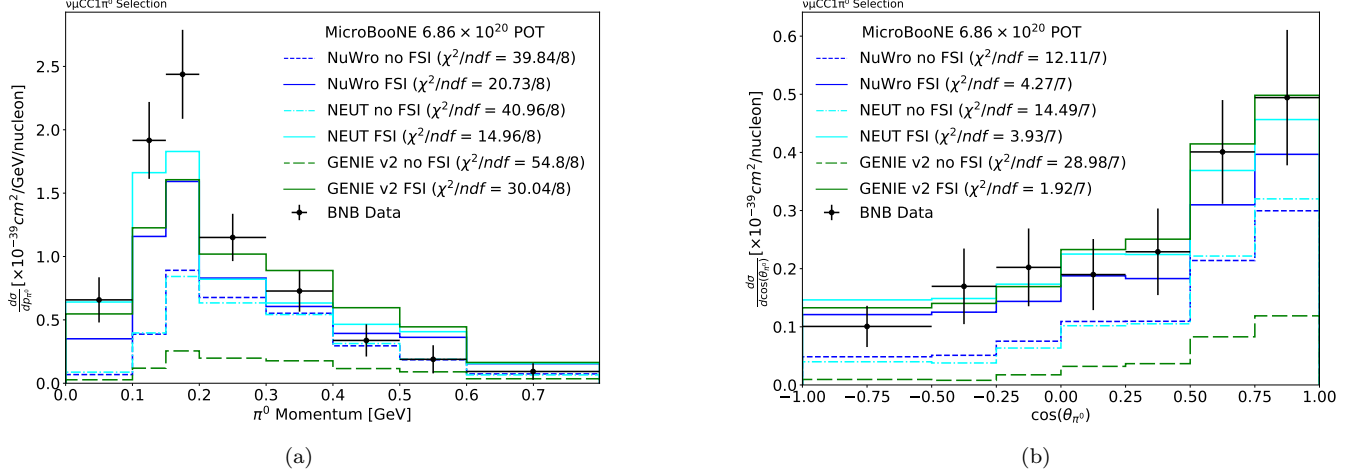

FIG. 24. Comparing differential cross sections from various generator predictions (with and without FSI effects) and the unfolded data for (a) the  $\pi^0$  momentum, (b) the scattering angle between the neutrino beam and outgoing  $\pi^0$  direction. We quantify the agreement in terms of  $\chi^2$  values, and list them in the legends.

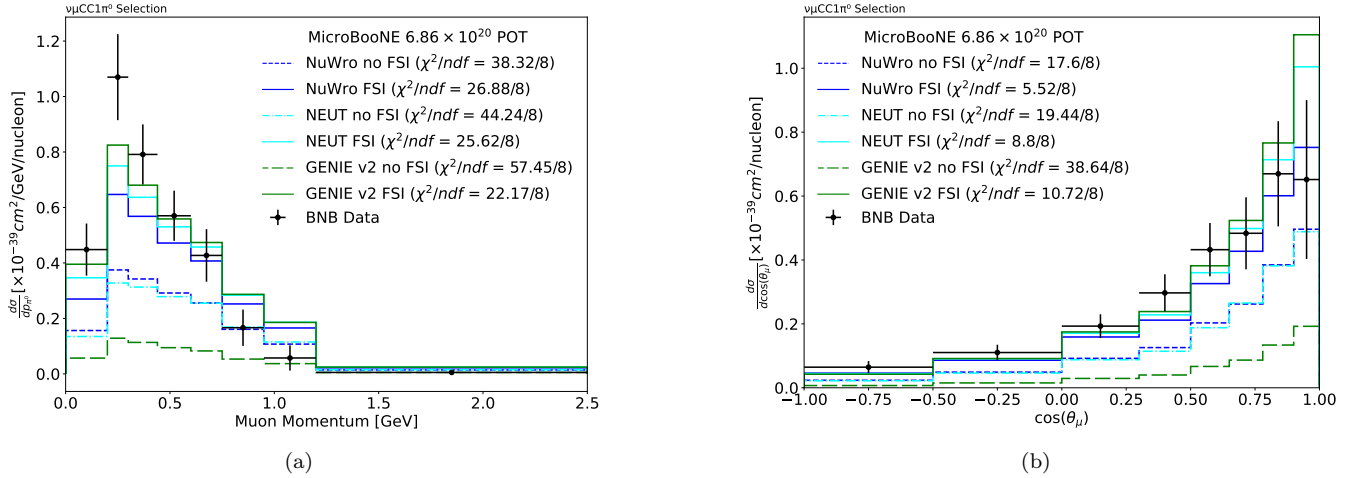

FIG. 25. Comparing differential cross sections from various generator predictions (with and without FSI effects) and the unfolded data for (a) the muon momentum, (b) the scattering angle between the neutrino beam and outgoing muon direction. We quantify the agreement in terms of  $\chi^2$  values, and list them in the legends.

- [1] P. Abratenko *et al.* (MicroBooNE Collaboration), First measurement of inclusive muon neutrino charged current differential cross sections on argon at  $E_\nu \sim 0.8$  GeV with the microboone detector, *Phys. Rev. Lett.* **123**, 131801 (2019).
- [2] C. Adams *et al.* (The MicroBooNE Collaboration), First measurement of  $\nu_\mu$  charged-current  $\pi^0$  production on argon with the microboone detector, *Phys. Rev. D* **99**, 091102 (2019).

- <sup>83</sup> [3] P. Abratenko *et al.* (MicroBooNE Collaboration), New CC0 $\pi$  genie model tune for microboone, [Phys. Rev. D](#) **105**, 072001  
<sup>84</sup> (2022).
